# Supplementary material for: Performance evaluation of the 8-inch MCP-PMT for Jinping Neutrino Experiment
Source: arXiv:2303.05373 source file (2023-03-09)
Supplement: Supplementary file 1 [file Appendix.tex]

\section{Weighted least square(WLS) for PDE}
\label{sec:solution}
\subsection{Single reference PMT}
\label{sec:singlepmt}
When the PMTs rotate in container for K times, $N=K$ and matrix D contains $NK=K^2$ rows:
\begin{equation}
    \bordermatrix{
        k&I&\alpha&\eta\cr
        0&\mathrm{I}_{(N,N)}&A_{0}&E_{0}\cr
        \vdots&\vdots&\vdots&\vdots\cr
        K-1&\mathrm{I}_{(N,N)}&A_{n}&E_{n}
    }
\end{equation}
in which $A_n$ and $E_n$ are in shape $(K,K-1)$. $A_n$ meet the condition $\sum_i{A_n[i,j]}=1$
\begin{equation}
    A_0=\begin{pmatrix}
        0\\
        I_{(K-1,K-1)}
    \end{pmatrix}
\end{equation}
and $A_n$ are the row arrangement of $A_0$ dependent on the test setting.

Due to the arrangement of $A_n$, each $A_n$ represent all test data for one PMT, therefore $E_n$ should match $A_n$ and all elements are 0 for $E_0$ or contans a column of 1.
\begin{equation}
    E_1=\begin{pmatrix}
        1&0&\dots&0\\
        \vdots&0&\ddots&0\\
        1&0&\dots&0
    \end{pmatrix}
\end{equation}
$E_n$ meet the condition $\sum_n{\sum_i{E_n[i,j]}}=J$.

Above is a special case when all tests contain same PMTs. The number of parameter must be smaller than equations, which lead to $(N-2)(K-1)\geq0$. This methods can be extends to more complicates situation, for example different runs may contain different PMTs. However, there are some limits. If no pmts are include in two different runs sets, $X$ can be split into 5 groups $X=[X_\alpha, X^1_I,X^2_I,X^1_\eta,X^2_\eta]$. The matrix D can be diagonalized into 3 matrix. 
\begin{equation}
    \begin{pmatrix}
        D^1_\alpha&D^1_I&D^1_\eta&0&0\\
        D^2_\alpha&0&0&D^2_I&D^2_\eta
    \end{pmatrix}
\end{equation}
Assume reference PMT exists in 1st group, if there exisit a solution or solution for minimum likelihood $[x_\alpha,x^1_I,x^2_I,x^1_\eta,x^2_\eta]$, $[x_\alpha,x^1_I,x^1_\eta,kx^2_I,x^2_\eta/k]$ will also be the solution, which means the $X^2_\eta$ can not be calculated.
\subsection{Two reference PMTs}
Assume one reference PMT fixed in 0th channel, the other reference PMT moved with test PMTs. Note the fixed reference PMT is Kth PMT, ids of other PMTs are same as . Matrix D contains $N(K+1)$ rows:
\begin{equation}
    \bordermatrix{
        k&I&\alpha_f\eta_f&\alpha_m&\eta_m\cr
        K&\mathrm{I}_{(N,N)}&1&0&0\cr
        0&\mathrm{I}_{(N,N)}&0&A_{0}&E_{0}\cr
        \vdots&\vdots&0&\vdots&\vdots\cr
        K-1&\mathrm{I}_{(N,N)}&0&A_{n}&E_{n}
    }=\begin{pmatrix}
        I&A_f&0\\
        B_m&0&A_m
    \end{pmatrix}
\end{equation}
in which $\alpha_f\eta_f$ is channel ratio multiplied by PDE of fixed PMT. Definition of $A_n$ and $E_n$ are same as Appendix~\ref{sec:singlepmt}. $X$ is splitted into 4 group, $X=[X_I,X^f_\eta,X^m_\alpha,X^m_\eta]$.

Assume PMTs are moved for $J$ times, the PDE $Q_j$ of test PMT can be calculated directly using
\begin{equation}
    \frac{Q_k}{Q_0} = \frac{R_{njk}R_{mJK}}{R_{mj0}R_{nJK}}
\end{equation}
variance of $R$ is Eq.~\eqref{equ:variance}, the relative variance of $\frac{Q_k}{Q_0}$ is $\sum_{i=jk,j0,JK,JK}{\frac{1-p_k}{N_tp_k}}$, in which $N_t$ is number of total events for some run. To get the PDE, a estimator is constructed as 
\begin{equation}
    \hat{\frac{Q_k}{Q_0}}=\frac{1}{N}\sum_j{\frac{R_{njk}R_{mJK}}{R_{mj0}R_{nJK}}}
\end{equation}
The relative variance of $\hat{\frac{Q_k}{Q_0}}$ can be estimated as $\frac{1}{J^2}\sum_k{\frac{1-p_k}{N_tp_k}}$. To be convenience, $p_k$s are close and note $\sigma^2=\frac{1-p_k}{N_tp_k}$, relative variance is $\frac{\sigma^2}{K}$

As for WLS method, the expected value and variance of $log(\hat{\frac{Q_k}{Q_0}})$ is estimated using Eq.~\eqref{equ:solution} and relative variance of $\hat{\frac{Q_k}{Q_0}}$ is estimated as $U=B\Sigma B^T=(D^T\Sigma D)^{-1}$.
\begin{equation}
    D^TD=\begin{pmatrix}
        (K+1)I_{(N,N)} &[1,\dots,1]^T&B_m^TA_m\\
        [1,\dots,1]&K&0\\
        A_m^TB_m&0&A_m^TA_m
    \end{pmatrix}
\end{equation}

In addition,
\begin{equation}
    A_m^TA_m=\begin{pmatrix}
        KI&1\\
        1&KI
    \end{pmatrix},
    A_m^TB_m=\begin{pmatrix}
        1\\
        1
    \end{pmatrix}
\end{equation}
Due to $det(D^TD)=$

If omit the non-diagonal elements, the variance of $\hat{\frac{Q_k}{Q_0}}$ is $\frac{\sigma^2}{K}$.
